# Supplementary material for: GOOSE: Goal-Conditioned Reinforcement Learning for Safety-Critical Scenario Generation
Source: arXiv:2406.03870 source file (2024-06-06)
Supplement: Supplementary file 1 [file A_appendix.tex]

\section*{APPENDIX}
